# Supplementary material for: Temporal-Logic-Based Reward Shaping for Continuing Reinforcement Learning Tasks
Source: arXiv:2007.01498 source file (2023-01-16)
Supplement: Supplementary file 1 [file supplementary.tex]

\subsection{Grid World}
\commenty{Move to supplementary}

\begin{figure}[h]
    \centering
    \subfloat[Gridworlds with and without a wall (in red) and with the state label $G$ in two different positions. ]{\input{figures/simple_gridworld}}
    \subfloat[Domain knowledge DFA]{\begin{tikzpicture}
		\node[state, initial left]  (q0) {$q_I$};
			\node[state,accepting] [above right= 0.15cm and 1 cm of q0] (q1) {$q_1$};
			\node[state] [below right= 0.15 and 1 cm of q0] (q2) {$q_2$};
% 			\node[state, accepting] [right=of q1] (q3) {$q_3$};
% 			\node[state] [right=of q2] (q4) {$q_4$};
			\draw 
			[->] (q0) edge node[above, sloped] {\tiny$\lnot G$} (q2)
% 			(q0) edge[bend right=80] node[below, sloped] {\tiny$cr \wedge ! (g1 \wedge g2)$} (q4)
			(q0) edge node[above, sloped] {\tiny $G$} (q1)
			(q1) edge node[right] {\tiny $\lnot G$} (q2)
			(q1) edge[loop right] node[right] {\tiny $G$} (q1)
			(q2) edge[loop right] node[right] {\tiny $\lnot G$} (q2);

\end{tikzpicture}}
    \caption{Variations on the gridworld case study from~\citep{mahadevan1996average}. Agent receives a reward when it moves to the green cell and is then transported to a random cell.}
    \label{fig:gridworld_setup}
\end{figure}

We compare our method against standard R-Learning in a Grid World environment as studied in~\citep{mahadevan1996average}. Figure~\ref{fig:gridworld_setup} shows the 6*6 grid with a +100 reward in the green cell. The agent moves one step in one of the four directions at every step, and gets ``transported'' to a random cell when it reaches the green cell.

The following four methods are compared: shielding, directly specified reward shaping, temporal-logic-based reward shaping, and baseline R-learning. %\suda{I think we remove the state based shaping, it's not necessary and doesn't add to the message} \commenty{The original reward shaping paper had this experiment, so it makes sense to show our shaping function is no worse than the original one.}

%\commenty{Describe temporal logic in notations defined in Sec. 4. Summarize learning parameters.}

The correctness of the expert knowledge is varied by adding the wall from (2, 2) to (2, 5) as shown in Figure~\ref{fig:gridworld_setup}, and moving the known reward position to (3, 3). \suda{Does the actual reward move or does our knowledge move?}
We conduct experiments in four conditions: no wall and correct position, no wall and wrong position, with wall and correct position, and with wall and wrong position. 

\begin{figure*}[h]
    \begin{subfigure}{.5\textwidth}
        \centering
        \includegraphics[width=.9\linewidth]{figures/simple.png}
        \caption{Simple grid world.}
    \end{subfigure}
    \begin{subfigure}{.5\textwidth}
        \centering
        \includegraphics[width=.9\linewidth]{figures/wall.png}
        \caption{Grid world with wall.}
    \end{subfigure}
    \newline
    \begin{subfigure}{.5\textwidth}
        \centering
        \includegraphics[width=.9\linewidth]{figures/wrong_distance.png}
        \caption{Grid world with inaccurate knowledge.}
    \end{subfigure}
    \begin{subfigure}{.5\textwidth}
        \centering
        \includegraphics[width=.9\linewidth]{figures/wrong_distance_and_wall.png}
        \caption{Grid world with wall and inaccurate knowledge.}
    \end{subfigure}
    \caption{Learning curves of temporal-logic-based reward shaping, directly specified reward shaping, shielding, and baseline in four conditions. Each condition is repeated 100 times.\suda{we should remove the state shaping from these graphs}} \commenty{We can cut (c) and (d) to save space.}
    \label{fig:gridworld}
\end{figure*}

Figure~\ref{fig:gridworld} shows the average reward received by each of the method in a sliding window of 100 steps, averaged by 100 runs. As expected, the hard shield performs optimally from the beginning when there is no wall and accurate knowledge of the reward cell, and fails to converge to the optimal policy in other conditions. The directly specified shaping method does not outperform our method in all four conditions, showing no benefit of the more complex potential function. Further, the shaping methods still outperform the R-learning baseline with inaccurate knowledge.
